# Supplementary material for: A Localized-Orbital Energy Evaluation for Auxiliary-Field Quantum Monte Carlo
Source: arXiv:2202.00832 ancillary file (2022-04-04)
Supplement: Supplementary file 1 [file Supplemental_Info.pdf]

# A Localized-Orbital Energy Evaluation for Auxiliary-Field Quantum Monte Carlo

John L. Weber,*,† Hung Vuong,† Pierre A. Devlaminck,† James Shee,‡ Joonho Lee,† David R. Reichman,† and Richard A. Friesner*,†

†*Department of Chemistry, Columbia University, 3000 Broadway, New York, NY, 10027*

‡*Kenneth S. Pitzer Center for Theoretical Chemistry, Department of Chemistry, University of California, Berkeley, California 94720, USA*

E-mail: jlw2245@columbia.edu; raf8@columbia.edu

## Supporting Information Available

## S1 MS Algorithm

Mahajan and Sharma (MS) have recently developed an algorithm for evaluating the two-body local energy for multideterminant trials which takes advantage of the rank $\epsilon$ excitation structure of CI expansions in a general way.[1,2] Here we reproduce key algorithmic details of this approach in our notation for clarity. The trial wavefunction is represented first as an expansion of excitation operators operating on the reference

$$|\Psi\rangle = \sum_{d}^{N_{det}} c_d \prod_{\mu_d}^{\epsilon_d} a^{\dagger}_{t_{\mu_d}} a_{p_{\mu_d}} |\psi_0\rangle, \tag{1}$$

where the operators $a^{\dagger}_{t_{\mu_d}} a_{p_{\mu_d}}$ excite a configuration from the occupied orbital $p_\mu$ into $t_\mu$, and $\epsilon_d$ denotes the number of excitations for the determinant indexed by the label $d$.

One can choose to rearrange the local energy as

$$E = \frac{\langle \Phi_T | \hat{H} | \Phi \rangle}{\langle \Phi_T | \Phi \rangle} = \frac{\langle \Psi | \hat{H} | \Phi \rangle}{\langle \psi_0 | \Phi \rangle} \Big/ \frac{\langle \Psi | \Phi \rangle}{\langle \psi_0 | \Phi \rangle}, \tag{2}$$

$$E = \frac{\sum_d^{N_{det}} c_d \langle \psi_0 | \prod_{\mu_d} a^\dagger_{p_{\mu_d}} a_{t_{\mu_d}} \hat{H} | \Phi \rangle}{\langle \psi_0 | \Phi \rangle} \Big/ \frac{\sum_d^{N_{det}} c_d \langle \psi_0 | \prod_{\mu_d} a^\dagger_{p_{\mu_d}} a_{t_{\mu_d}} | \Phi \rangle}{\langle \psi_0 | \Phi \rangle}, \tag{3}$$

where the overlap ratios in the denominator can be computed with $\mathcal{O}(N^2 M + N_{det})$ cost if one works in the MO basis, and $\mathcal{O}(NM^2 + N_{det})$ cost if not.[2] Skipping the one body contribution, which can be calculated at a similar cost, we then rewrite the resulting two body energy contribution in terms of the reference CI determinant,

$$E_2 = \sum_d^{N_{det}} c_d \cdot \frac{1}{2} \sum_{pqrs}^{M} \sum_{\alpha}^{X} L^{\alpha}_{rp} L^{\alpha}_{sq} \frac{\langle \psi_0 | (\prod_{\mu_d} a^\dagger_{p_{\mu_d}} a_{t_{\mu_d}}) a^\dagger_p a^\dagger_q a_r a_s | \phi \rangle}{\langle \psi_0 | \phi \rangle}. \tag{4}$$

The generalized Wick's theorem enables the expansion of this term as a function of the reference Green's function. Dropping the determinant index $d$, we find

$$\frac{\langle \psi_0 | \prod_{\mu_d} a^\dagger_{p_{\mu_d}} a_{t_{\mu_d}} a^\dagger_p a^\dagger_q a_r a_s | \phi \rangle}{\langle \psi_0 | \phi \rangle} = \det \begin{pmatrix} G^{\{p,q\}}_{\{r,s\}} & \mathcal{G}^{\{p,q\}}_{\{t_\mu\}} \\ G^{\{p_\mu\}}_{\{r,s\}} & G^{\{p_\mu\}}_{\{t_\mu\}} \end{pmatrix} = \det \begin{pmatrix} G_{pr} & G_{ps} & \mathcal{G}_{p\{t_\mu\}} \\ G_{qr} & G_{qs} & \mathcal{G}_{q\{t_\mu\}} \\ G_{\{p_\mu\}r} & G_{\{p_\mu\}s} & G_{\{p_\mu\}\{t_\mu\}} \end{pmatrix}, \tag{5}$$

where $\mathbf{G}$ is the Green's function associated with the reference determinant, calculated at cost $N^2 M$ in the MO basis, and the sets $\{p_\mu\}$ and $\{t_\mu\}$ are the $\epsilon$ occupied and virtual excitation orbitals for the particular determinant. $\mathcal{G}_{ab}$ is defined as $\mathcal{G}_{ab} = G_{ab} - \delta_{ab}$. This expression can then be Laplace expanded across the first two columns, yielding the following equation for the determinant in Eq. 5,

$$det \begin{pmatrix} G^{\{p,q\}}_{\{r,s\}} & \mathcal{G}^{\{p,q\}}_{\{t_\mu\}} \\ G^{\{p_\mu\}}_{\{r,s\}} & G^{\{p_\mu\}}_{\{t_\mu\}} \end{pmatrix} = [G_{pr}G_{sq} - G_{qr}G_{ps}]\text{det}(G_{\{p_\mu\}\{t_\mu\}})$$

$$+ \sum_{\nu}^{\epsilon}(-1)^{\nu}[G_{ps}G_{p_\nu r} - G_{pr}G_{p_\nu s}]\text{det}\begin{pmatrix} \mathcal{G}_{q\{t_\mu\}} \\ G_{\{p_{\mu\neq\nu}\}\{t_\mu\}} \end{pmatrix}$$

$$+ \sum_{\nu,\nu',\lambda,\lambda'}^{\epsilon}(-1)^{\nu+\nu'+\lambda+\lambda'}G_{p_\nu r}G_{p_{\nu'} s}\mathcal{G}_{pt_\lambda}\mathcal{G}_{qt_{\lambda'}}\text{det}(G_{\{t_{\mu\neq\{\nu,\nu'\}}\}\{p_{\mu\neq\{\lambda,\lambda'\}}\}}). \quad (6)$$

Plugging Eq. 6 into Eq. 4 results in an equation that allows for a separation of sums over Hamiltonian and determinant indices. For each determinant we have

$$E_2^d = E_2^0 \times \text{det}(G_{\{p_\mu\}\{t_\mu\}}) + \sum_{\nu}^{\epsilon}(-1)^{\nu}\text{det}\begin{pmatrix} [D_1]_{p_\nu\{t_\mu\}} \\ G_{\{p_{\mu\neq\nu}\}\{t_\mu\}} \end{pmatrix}$$

$$+ \sum_{\alpha}^{X}\sum_{\nu,\nu',\lambda,\lambda'}^{\epsilon}(-1)^{\nu+\nu'+\lambda+\lambda'}[[D_2]^{\alpha}_{p_\nu t_\lambda}[D_2]^{\alpha}_{p_{\nu'} t_{\lambda'}} - [D_2]^{\alpha}_{p_\nu t_{\lambda'}}[D_2]^{\alpha}_{p_{\nu'} t_\lambda}] \times \text{det}(G_{\{t_{\mu\neq\{\nu,\nu'\}}\}\{p_{\mu\neq\{\lambda,\lambda'\}}\}}), \quad (7)$$

where $E_2^0$, $[D_1]_{pt}$, and $[D_2]^{\alpha}_{pt}$ are expressed as

$$E_2^0 = \sum_{\alpha}^{X}\sum_{pqrs} L^{\alpha}_{rp}L^{\alpha}_{sq}[G_{pr}G_{qs} - G_{qr}G_{ps}],$$

$$[D_1]_{p_\mu t_\mu} = \sum_{\alpha}^{X}\sum_{pqrs} L^{\alpha}_{rp}L^{\alpha}_{sq}[G_{ps}G_{p_\mu s} - G_{pr}G_{p_\mu r}]\mathcal{G}_{qt_\mu},$$

$$[D_2]^{\alpha}_{p_\mu t_\mu} = \sum_{pr} L^{\alpha}_{rp}G_{p_\mu r}\mathcal{G}_{pt_\mu}. \quad (8)$$

These terms can be calculated at a cost of $XNM^2$, $XNAM$, and $XNAM$, respectively, where $A$ is the size of the active space. Note that for $[D_2]^{\alpha}_{p_\mu t_\mu}$, we have a partial summation of Hamiltonian indices, leaving the last term of Eq. 7 to be calculated at a cost of $N_{det}X$.

The resulting algorithm thus scales as $\mathcal{O}(N_{det}S + S^4)$, where $S$ is a general proxy for the system size. It is possible to precompute the sum over $\alpha$ as well, leading to an algorithm scaling as $\mathcal{O}(N_{det} + S^5)$, but this becomes intractable for even medium system sizes.

## S1.1 LO-AFQMC in the MS Algorithm

The compression of the HR-ERI tensor allows for two significant sources of improvement in scaling versus Eqns. 6-8. Firstly, the sum over auxiliary fields is precomputed and folded into the integrals. Savings due to this are additionally possible if one uses the full HR-ERIs, but at a prohibitive memory cost. Upon localization, that memory cost becomes insignificant, and we can additionally replace a factor of M with $\langle M_{SVD}\rangle$. The most straightforward applications are to $E_2^0$ and $[D_1]_{p_\mu t_\mu}$, which take the form of sums similar to Eq. 22, but for the reference determinant only,

$$E_2^0 = \sum_{ij}^{N} \sum_{K}^{M_{SVD}} \sum_{rs}^{M} \bar{U}_{rK}^{[ij]} \bar{V}_{Ks}^{[ij]} [Q_{ir}Q_{js} - Q_{jr}Q_{is}], \tag{9}$$

$$[D_1]_{p_\mu t_\mu} = \sum_{ij}^{N_{cas}} \sum_{K}^{M_{SVD}} \sum_{rs}^{M} \bar{U}_{rK}^{[ij]} \bar{V}_{Ks}^{[ij]} [Q_{is}Q_{p_\mu r} - Q_{ir}Q_{p_\mu s}] \mathcal{G}_{jt_\mu}. \tag{10}$$

The largest scaling step is the contraction over full basis indices $r$ and $s$, which scales as $\mathcal{O}(N^2 M\langle M_{SVD}\rangle)$, reducing the scaling from quartic to cubic. For the last term of Eq. 7, it is most advantageous to perform the summation of all four indices at once,

$$[D_3]_{p_\nu p_{\nu'} t_\lambda t_{\lambda'}} = \sum_{ij}^{N_{cas}} \sum_{K}^{M_{SVD}} \sum_{rs}^{M} \bar{U}_{rK}^{[ij]} \bar{V}_{Ks}^{[ij]} Q_{p_\nu r} Q_{p_{\nu'} s} \mathcal{G}_{it_\lambda} \mathcal{G}_{jt_{\lambda'}}. \tag{11}$$

Note that this is equivalent to $[D_3]_{p_\nu p_{\nu'} t_\lambda t_{\lambda'}} = \sum_\alpha^X [D_2]^\alpha_{p_\nu t_\lambda} [D_2]^\alpha_{p_{\nu'} t_{\lambda'}} - [D_2]^\alpha_{p_\nu t_{\lambda'}} [D_2]^\alpha_{p_{\nu'} t_\lambda}$ in Eq. 7, but using the localized HR-ERIs and changing the order of summation so that it is not necessary to explicitly form the set of $[D_2]^\alpha$. As all Green's functions in this Eq. are reference Green's functions, we can make use of the form outlined in section S3, and replace all general

indices $p$ and $q$ with occupied indices $i$ and $j$. The formation of this four index tensor of size $A_{occ}^2 A_{virt}^2$ now scales as $N^2 M A_{occ} \langle M_{SVD} \rangle$, where $A_{occ}$ and $A_{virt}$ are the number of occupied and virtual orbitals in the active space, respectively. $E_2$ can now be calculated as

$$E_2^d = E_2^0 \det(G_{\{p_\mu\}\{t_\mu\}}) + \sum_{\nu}^{\epsilon} (-1)^\nu \times \det \begin{pmatrix} [D_1]_{p_\nu \{t_\mu\}} \\ G_{\{p_{\mu \neq \nu}\}\{t_\mu\}} \end{pmatrix} + \sum_{\nu,\nu',\lambda,\lambda'}^{\epsilon} (-1)^{\nu+\nu'+\lambda+\lambda'} [D_3]_{p_\nu p_{\nu'} t_\lambda t_{\lambda'}} \times \det(G_{\{t_{\mu \neq \{\nu,\nu'\}}\}\{p_{\mu \neq \{\lambda,\lambda'\}}\}}). \quad (12)$$

This expression can then be used to calculate the energy at a cost of $\mathcal{O}(N_{det})$, with an overall scaling for the energy evaluation of $\mathcal{O}(N^2 M A_{occ} + N_{det})$.

# S2 Additional Details of GPU implementation

It is an unfortunate consequence of GPU architectures that operations involving lists of small matrices with inconsistent dimension are not easily parallelized. We therefore restrict $\epsilon$ to be equivalent to the maximum number of excitations, regardless of the number of excitations in that specific determinant, allowing these operations to be easily batched over $N_{det}$ using, for example, `cublas<T>gemmBatched()` functions. While it is possible to use a similar restriction in $M_{SVD}$, this would result in significant loss of memory and computational efficiency. We have found it possible to perform the largest scaling operations over $M_{SVD}$ for all $[ij]$ pairs concurrently by storing matrix lists contiguously in memory. An example of this difficulty can be seen in an intermediate step in the formation of the reference section of $\bar{Q}_{R,i}^{d,[ij]}$ (Eq. 31):

$$X_{L,i}^{[ij]} = \sum_r^M [\bar{U}_{rK}^{[ij]}] * [\Phi_{ra} A_{ai}^{-i}]. \quad (13)$$

Ideally, we would like to batch the sum over r for all [ij] pairs, all determinants, and all walkers at the same time. This is particularly difficult, as all [ij] pairs have a different

dimension of K. Additionally, the vector on the right hand side depends on i, and so batching is only possible for all [ij] pairs with a common i. Batching is enabled by storing $\bar{U}^{[ij]}_{rK}$ in memory as a contiguous list of matrices of size M by $M^{[ij]}_{SVD}$, with the pairs [ij] in "i major" format:

$$\underbrace{\bar{U}^{[0,0]}, \bar{U}^{[0,1]}, \ldots \bar{U}^{[0,N_{cas}]}}_{i=0}, \underbrace{\bar{U}^{[1,1]}, \bar{U}^{[1,2]}, \ldots \bar{U}^{[1,N_{cas}]}}_{i=1}, \ldots, \underbrace{\bar{U}^{[N_{cas},N_{cas}]}}_{i=N_{cas}}$$

The formation of a particular $X^{[ij]}_{L,i}$ then takes the form of a simple matrix-vector multiplication. Further parallelization is possible when the GPU is not saturated by taking advantage of CUDA streams.

We note that for the 'j' section, $\bar{Q}^{d,[ij]}_{L,j}$, we lose the contiguous nature of each i (aka all [ij] pairs with the same j are not contiguous). This is treated by a custom memory copying CUDA kernel, which takes all $\bar{U}^{[ij]}_{rK}$ with a given j and forms an intermediate tensor which is contiguous. As GPU memory copying is generally fast, this leads to a significant increase in performance, with the formation of $X^{[ij]}_{L,j}$ being 21.7 times faster than performing the matrix vector calls in series for benzene in the cc-pVTZ-DK basis. There is a similar step in the active section (last term on the right hand side) of equation 31; the rest of the operations can be performed in parallel for all pairs [ij].

## S3 Molecular orbital simplification

Large computational savings can be obtained by simply propagating in the basis of molecular orbitals for the trial, which we will often take advantage of in estimating scalings below. We briefly illustrate this here for clarity. When operating in the orthogonal MO basis, the matrix representing the trial wavefunction (namely the reference determinant in the case of CI expansions) can be written in block diagonal form,

$$\Phi_T = \left[\frac{I}{0}\right], \tag{14}$$

where $I$ is the $N$x$N$ identity matrix. We will now show that, as a result

$$Q = [\Phi(\Phi_T^\dagger\Phi)^{-1}] = \left[\begin{array}{c} I \\ \hline \Theta \end{array}\right]. \tag{15}$$

We denote the matrix representing a walker's antisymmetrized orbitals by

$$\Phi = \left[\begin{array}{c} K \\ \hline K' \end{array}\right]. \tag{16}$$

It follows that

$$(\Phi_T^\dagger\Phi)^{-1} = \left[\begin{array}{c} K^{-1} \end{array}\right], \tag{17}$$

and

$$Q = \Phi(\Phi_T^\dagger\Phi)^{-1} = \left[\begin{array}{c} K \\ \hline K' \end{array}\right] \left[\begin{array}{c} K^{-1} \end{array}\right] = \left[\begin{array}{c} KK^{-1} \\ \hline K'K^{-1} \end{array}\right] = \left[\begin{array}{c} I \\ \hline \Theta \end{array}\right]. \tag{18}$$

Now the Green's function takes the following form, where only a $(M-N)N$ block is significant, versus the $M^2$ significant elements in the atomic orbital (AO) basis,

$$\begin{array}{r} N \left\{ \vphantom{\mathbb{1}} \right. \\ (M-N) \left\{ \vphantom{G_{ai}} \right. \end{array} \left[\begin{array}{c:c} \overbrace{\quad\mathbb{1}\quad}^{N} & \\ \hdashline G_{ai} & 0 \end{array}\right]$$

where "$a$" denotes a virtual orbital, and "$i$" an occupied orbital. In the case of a CI expansion trial, this structure only remains for the inactive orbitals, and the active space results in mixing, with only the first $N_{cas}$ columns being nonzero, and the first $N_{inact} \times N_{inact}$ block

being the identity.

# S4 SMW algorithm for the formation of the Green's Function

Here we give details on the implementation and scaling of the formation of the Green's function for use in evaluating both the force bias and the 1-body energy. In contrast to the 2-body energy, we can perform the sum over determinants in the formation of the Green's function,

$$E_1 = \sum_{pr}^{M} \left[ \sum_{d}^{N_{det}} c_d G_{pr}^d \right] K_{pr} = \sum_{pr}^{M} \bar{G}_{pr} K_{pr} \tag{19}$$

where $K_{pr}$ are the 1-body integrals (or in the case of the force bias, $K_{pr}$ would be a Cholesky vector $L_{pr}^{\alpha}$). The summed Green's function $\bar{G}_{pr} = \sum_d^{N_{det}} c_d G_{pr}^d$ is in practice expanded via SMW along the lines of the $Q$ matrix written out in eq. 20,

$$\bar{G} = \sum_{d}^{N_{det}} Q^d c_d * \Phi_T^{d,\dagger} = \sum_{d}^{N_{det}} c_d \left[ \Phi A^{-1} \Phi_T^{d,\dagger} - \Phi A^{-1} U^d (I + V^{T,d} A^{-1} U^d)^{-1} V^{T,d} A^{-1} \Phi_T^{d,\dagger} \right]. \tag{20}$$

Since we can now include the sum over determinants in this expression (as was not the case when forming the intermediate Q matrices for the 2-body energy), we can rewrite this as

$$\bar{G} = \sum_{d}^{N_{det}} c_d \left[ \Phi A^{-1} \Phi_T^{d,\dagger} \right] - \sum_{d}^{N_{det}} c_d \left[ \Phi A^{-1} U^d (I + V^{T,d} A^{-1} U^d)^{-1} V^{T,d} A^{-1} \Phi_T^{d,\dagger} \right], \tag{21}$$

$$= \Phi A^{-1} \sum_{d}^{N_{det}} c_d \left[ \Phi_T^{d,\dagger} \right] - \Phi A^{-1} \sum_{d}^{N_{det}} c_d \left[ U^d (I + V^{T,d} A^{-1} U^d)^{-1} V^{T,d} A^{-1} \Phi_T^{d,\dagger} \right] \tag{22}$$

If propagating in the MO basis, $\Phi_T^{d,\dagger}$ has a form of identity plus some permutation,

rendering all operations involving it trivial memory transfers, and thus the reference term (first term of right hand side of 22) scales as $\mathcal{O}(MN^2)$. In Table S1 we outline key steps and scaling involved in evaluating the rightmost term, the correction term.

Table S1: List of key intermediates in the formation of the Green's function using SMW, including the formal memory and computational scaling of forming them. $N^a_{occ}$ and $N^a_{unocc}$ refer to the number of occupied orbitals in the active space and number of unoccupied orbitals in the active space, respectively.

| Intermediate | Operation | Memory scaling | Computational scaling |
|---|---|---|---|
| $C_1 = V^{T,d}A^{-1}$ | $V^{T,d} \times A^{-1}$ | $N_{det}N\epsilon$ | $\min(N_{det}N^2\epsilon,\ N^2N^a_{occ}N^a_{unocc})$ |
| $C_2 = (I + V^{T,d}A^{-1}U^d)^{-1}$ | Inverse | $N_{det}\epsilon^2$ | $N_{det}\epsilon^3$ |
| $C_3 = (I + V^{T,d}A^{-1}U^d)^{-1}V^{T,d}A^{-1}$ | $C_2 \times C_1$ | $N_{det}N\epsilon$ | $N_{det}N\epsilon^2$ |

Note that the $\epsilon$ by $N$ matrices $U^d$ and $V^{T,d}$ have structures that can lead to increased savings. If $N_{inact}$ is the number of inactive occupied orbitals, the first $N_{inact}$ rows of $U^d$ are zero, whereas the rest are either identity or a permutation matrix corresponding to the excitation structure of the determinant. Thus, the operation $U^d \times C_3$ would involve taking the last $N - N_{inact}$ rows of $C_3$ and performing some memory transfers, similar to how operations involving the trial determinants reduce to memory transfers when in the MO basis. $V^{T,d}$, while being a dense matrix, consists of a series of rows each corresponding to a single excitation from orbital a to b, $c_b^\dagger c_a$. While there may be many determinants in the CI expansion which have a given excitation, there are only $N^a_{occ}N^a_{unocc}$ possible single excitations, and one must only compute the rows of $C_1$ for each excitation once, maximally scaling as $N^2N^a_{occ}N^a_{unocc}$ in the case where all possible excitations are present in the CI expansion. Including all steps outlined here, the formal scaling of the formation of the Green's function in the MO basis is $\mathcal{O}(N^2(M+N^a_{occ}N^a_{unocc})+N_{det}N)$. For CAS trials, which become intractable over about 18 orbitals, $N^a_{occ}N^a_{unocc}$ is typically much smaller than the basis size M. Once the Green's function is formed, the 1-body energy can be evaluated at cost $M^2$, and the force bias with cost $XM^2$. We note that it is likely possible to extend the savings due to compression to the evaluation of the force bias, but as this would neither reduce the formal scaling of the overall AFQMC nor reduce the memory overhead (as one still requires the full cholesky vectors to compute the propagation matrix $\sum_\alpha^X x_\alpha L^\alpha$ at cost $XM^2$), we do not explore this

further.

## S5 LO error cancellation through imaginary time

Plotting LO errors over multiple time steps is made difficult by population control, which can be sensitive to small deviations in the energy (and thus weight) and mask the error due to the LO approximation with the intrinsic variance of AFQMC. We thus propagated 20 independent walkers for 100 $Ha^{-1}$ (Fig. S1), evaluating the mean and standard deviation at every step for $C_8H_8$, the platonic hydrocarbon which exhibited the greatest difference in error between the two times steps in Figure 7. The variance of the LO error over imaginary time then leads to the slight increase in statistical error mentioned in the main text. Note that the error does not increase dramatically as a function of imaginary time.

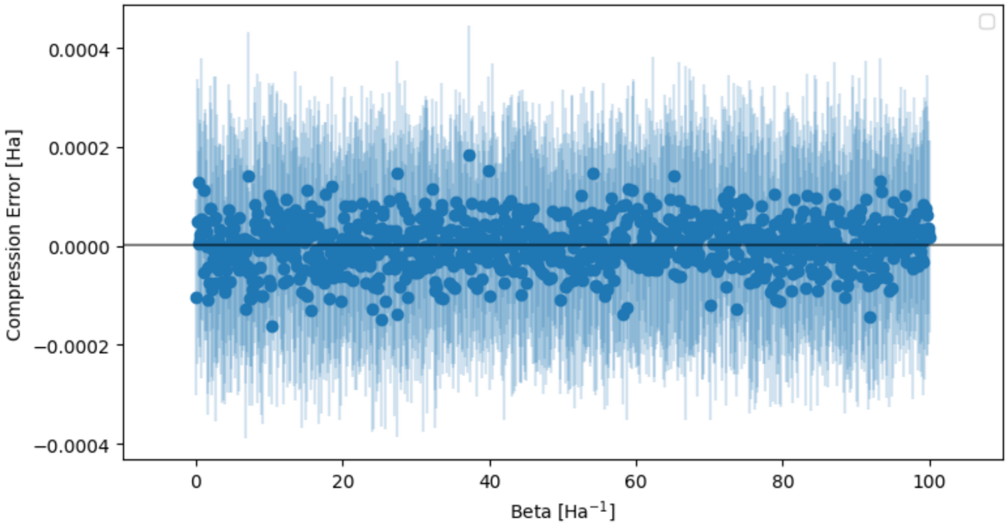


Figure S1: Plot of the mean and statistical error of the LO error of a set of 20 independent walkers for the system $C_8H_8$. The error exhibits a variance which contributes minimally to the statistical error, and does not grow significantly in imaginary time. The mean error in this case was 0.002 mHa, with a standard deviation of 0.2 mHa, representing a favorable cancellation of error over imaginary time.

# References


(1) Mahajan, A.; Sharma, S. Efficient local energy evaluation for multi-Slater wave functions in orbital space quantum Monte Carlo. *The Journal of Chemical Physics* **2020**, *153*, 194108.

(2) Mahajan, A.; Sharma, S. Taming the Sign Problem in Auxiliary-Field Quantum Monte Carlo Using Accurate Wave Functions. *Journal of Chemical Theory and Computation* **2021**, *17*, 4786–4798.
